# Supplementary material for: Kinetics of lithium electrodeposition and stripping
Source: arXiv:2008.00112 source file (2020-07-31)
Supplement: Supplementary file 1 [file SI.pdf]

# Supplementary Information:
# Kinetics of lithium electrodeposition and stripping


Shashank Sripad* and Venkatasubramanian Viswanathan†

*Department of Mechanical Engineering, Carnegie Mellon University, Pittsburgh, Pennsylvania 15213*

Daniel Korff* and Steven C. DeCaluwe

*Department of Mechanical Engineering, Colorado School of Mines, Golden, Colorado, 80401*



(Dated: July 31, 2020)


## 1. FITTING RESULTS FOR THE SOLVENTS

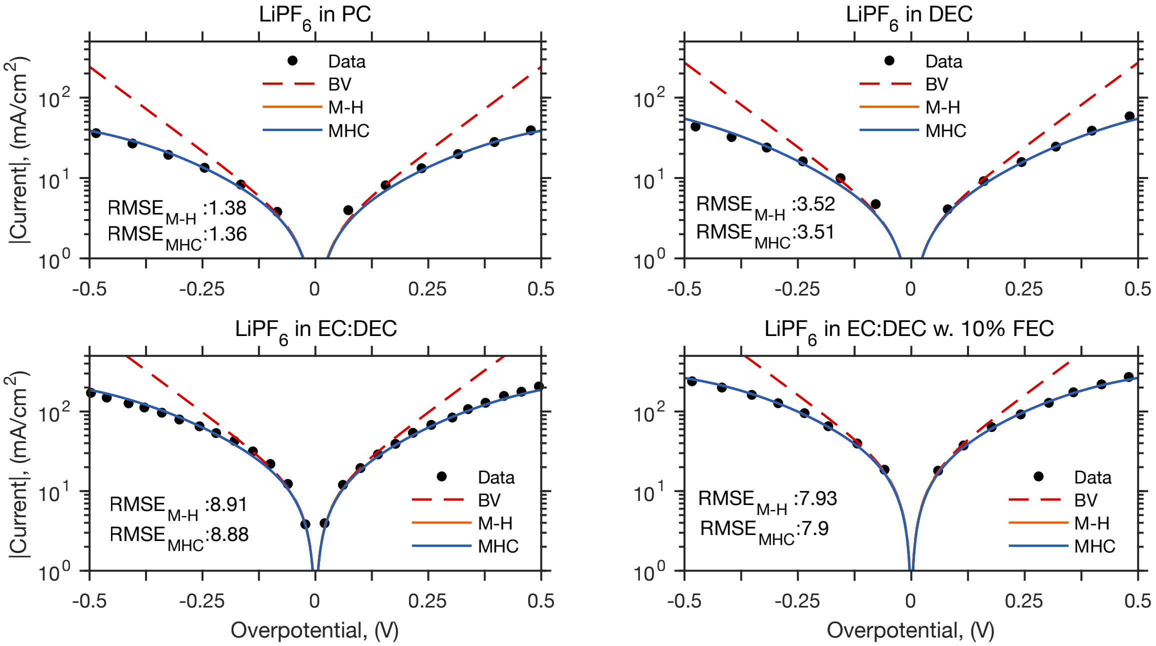


FIG. 1. The predictions of current density as provided by the BV model, the M-H model (proposed by Boyle *et. al*)[1] and the MHC model for four different solvents, namely, a. PC, b. DEC, c. EC:DEC, d. EC:DEC w. 10% FEC. This accompanies Figure 1. in the manuscript. Here we observe that within an overpotential region of 0.25V, the M-H model and the MHC model collapse on each other.

* These two authors contributed equally
† venkvis@cmu.edu

[1] D. T. Boyle, X. Kong, A. Pei, P. E. Rudnicki, F. Shi, W. Huang, Z. Bao, J. Qin, and Y. Cui, ACS Energy Lett. **5**, 701 (2020).
